# Supplementary material for: Hyperbolic VAE via Latent Gaussian Distributions
Source: arXiv:2209.15217 source file (2023-10-29)
Supplement: Supplementary file 1 [file 06_NumericalStability.tex]

\section{Numerical Stability}
\label{apx:numerical_stability}
We conduct an analysis of the numerical stability of the PGM normal distribution compared to the HWN and Poincar\'e normal. 
During the density estimation experiment, the HWN VAE and Poincar\'e VAE are often shown to be numerically unstable and fail to run in binarized-Breakout. Similar observations have been reported in several previous works ~\citep{mathieu19, fhnn, MVAE}.

The hyperbolic wrapped normal uses the exponential map when transforming the output of the encoder to the Lorentz model and during the sampling, as described in \autoref{eq:wrapped_normal}.
The overlapped Lorentz model exponential map often causes an overflow due to the hyperbolic functions in the exponential map such as $\cosh$ and $\sinh$.
Note that the hyperbolic functions exponentially grow with the positive input value.

In the training of Poincar\'e VAE, the KL divergence between the variational distribution and the prior distribution needs to be approximated by the log-probability of the samples due to the absence of closed-form KL divergence in Poincar\'e normal.
To compute the log probability of a given sample, the distance between two Poincar\'e disk model points, the sample and the Fr\'echet mean of the distribution needs to be calculated, where the distance function of the Poincar\'e disk model is defined as:
\begin{equation}
    d^c_{\mathcal{P}}(\rvx, \rvy) = \frac{1}{\sqrt{c}} \cosh^{-1}\left(1 + 2c \frac{\Vert \rvx - \rvy \Vert^2}{(1 - c\Vert \rvx \Vert^2)(1 - c\Vert \rvy \Vert^2)} \right),
\end{equation}
where $\Vert \cdot \Vert$ is the Euclidean norm.
The denominator term is unstable when $\Vert \rvx \Vert$ or $\Vert \rvy \Vert$ is close to value $\frac{1}{\sqrt{c}}$, which occurs when $\rvx$ and $\rvy$ are near the border of the Poincar\'e disk.

PGM normal, on the other hand, the KL divergence between an arbitrary PGM normal and $\mathcal{K}_c(\boldsymbol{0}, I, I)$, which is the only operation used during the training of GM-VAE, can be stably computed using the log-covariance.
For example, the KL divergence between a univariate Gaussian distribution $\mathcal{N}(\mu, \sigma)$ and the prior distribution mentioned above written as \autoref{eq:kl_divergence} can be computed with $\log \sigma^2$.
The KL divergence between two Gamma distributions, $\textrm{Gamma}(a_1, b_1)$ and $\textrm{Gamma}(a_2, b_2)$, written as:
\begin{equation}
    \KL(\textrm{Gamma}(a_1, b_1) \parallel \textrm{Gamma}(a_1, b_1)) = a_2 \log \frac{b_1}{b_2} - \ln \frac{\Gamma(a_1)}{\Gamma(a_2)} + (a_1 - a_2) \psi(a_1) - (1 - \frac{b_2}{b_1}) a_1,
\end{equation}
where $\psi$ is the digamma function, can be stablly computed using $\log b_1$ when $b_1$ is large due to small $\beta$ and $\gamma$ in the factorization \autoref{eq:factorization}.
