# Supplementary material for: Hyperbolic VAE via Latent Gaussian Distributions
Source: arXiv:2209.15217 source file (2023-10-29)
Supplement: Supplementary file 2 [file Isometries.tex]

\section{Operations of the Hyperbolic Spaces}
\label{apx:geometric_transformations}

\subsection{Isometries}
In this section, we derive the isometries between the two-dimensional hyperbolic models, the Lorentz model, the Poincar\'e disk model and the Gaussian manifold with arbitrary curvatures.
Isometry between the Poincar\'e disk model and the Lorentz model $T_{\mathcal{L}_c \rightarrow \mathcal{P}_c}: \mathcal{L}_c \rightarrow \mathcal{P}_c$ is computed as:
\begin{equation*}
    T_{\mathcal{L}_c \rightarrow \mathcal{P}_c}((t, x, y)) = \left(\frac{x}{\sqrt{c}t + 1}, \frac{y}{\sqrt{c}t + 1}\right),
\end{equation*}
and the inverse is:
\begin{equation}
    T^{-1}_{\mathcal{L}_c \rightarrow \mathcal{P}_c}((x, y)) \left( \frac{1 + (x^2 + y^2)c}{\sqrt{c} (1 - (x ^2 + y^2)c)}, \frac{2x}{1 - (x ^2 + y^2)c}, \frac{2y}{1 - (x ^2 + y^2)c} \right).
\end{equation}

Isometry between the Gaussian manifold and the Poincar\'e disk model $T_{\mathcal{P}_c \rightarrow \mathcal{U}_c}: \mathcal{P}_c \rightarrow \mathcal{U}_c$ is computed as:
\begin{equation*}
    T_{\mathcal{P}_c \rightarrow \mathcal{G}_c}(x, y) = \left( \frac{-2y}{(\sqrt{c}x - 1)^2 + y^-2c}, \frac{1 - (x^2 + y^2)c}{(\sqrt{c}x - 1)^2 + y^-2c} \right), 
\end{equation*}
and the inverse is:
\begin{equation}
     T^{-1}_{\mathcal{P}_c \rightarrow \mathcal{G}_c}(x, y) \left( \frac{\sqrt{c}x^2 + (y^2 - 1) / \sqrt{c}}{cx^2 + (y + 1)^2}, \frac{-2x}{cx^2 + (y + 1)^2} \right).
\end{equation}

Finally, the isometry between the Gaussian manifold and the Lorentz model $T_{\mathcal{L}_c \rightarrow \mathcal{G}_c}$ can be derived by composing $T_{\mathcal{L}_c \rightarrow \mathcal{P}_c}$ and $T_{\mathcal{P}_c \rightarrow \mathcal{G}_c}$ as:
\begin{equation*}
    T_{\mathcal{L}_c \rightarrow \mathcal{G}_c}(t, x, y) = \left( \frac{-y}{\sqrt{c}(t-x)}, \frac{1}{\sqrt{c}(t - x)} \right), 
\end{equation*}
and the inverse is:
\begin{equation}
    T^{-1}_{\mathcal{L}_c \rightarrow \mathcal{G}_c}(x, y) = \left( \frac{1 + cx^2 + y^2}{2\sqrt{c}y}, \frac{-1 + cx^2 + y^2}{2\sqrt{c}y}, -\frac{x}{y}\right).
\end{equation}

We then empirically show that the isometries preserve the distance between the points when transformed to other models.
We randomly sampled 1,000 pairs of Gaussian manifold points with range of $\mu \in [-100, 100]$ and $\sigma \in [0, 100]$. We report the average difference in the distance for each pair before the transformation and after the transformation. We vary the curvature value from 0.25 to 2.
For the Gaussian manifold, we use the following distance function for arbitrary curvature:
\begin{equation*}
    d_{\mathcal{U}_c}((x_1, y_1), (x_2, y_2)) = \frac{1}{\sqrt{c}}\log \frac{\sqrt{c(x_1 - x_2)^2 + (y_1 + y_2)^2 } + \sqrt{c(x_1 - x_2)^2 + (y_1 - y_2)^2}}{\sqrt{c(x_1 - x_2)^2 + (y_1 + y_2)^2} - \sqrt{c(x_1 - x_2)^2 + (y_1 - y_2)^2}}.
\end{equation*}
\autoref{tab:isometry_validation} shows that the proposed isometries well-preserve the distances.

\begin{table}[h!]
    \centering
    \caption{Validation of the proposed isometries between the hyperbolic models.}
    \label{tab:isometry_validation}
    \begin{tabular}{r c c c}
        \toprule
        $c$
        & $T_{\mathcal{P}_c \rightarrow \mathcal{L}_c}$
        & $T_{\mathcal{G}_c \rightarrow \mathcal{P}_c}$
        & $T_{\mathcal{G}_c \rightarrow \mathcal{L}_c}$
        \\
        \midrule
        0.25 & $5.72\textrm{e}{-13}$& $1.50\textrm{e}{-13}$& $4.76\textrm{e}{-13}$\\
        0.50 & $8.41\textrm{e}{-13}$& $3.10\textrm{e}{-13}$& $6.23\textrm{e}{-13}$\\
        1.00& $7.84\textrm{e}{-13}$& $4.22\textrm{e}{-13}$& $4.88\textrm{e}{-13}$ \\
        1.50& $3.22\textrm{e}{-12}$& $2.51\textrm{e}{-12}$& $8.30\textrm{e}{-13}$ \\
        2.00& $1.89\textrm{e}{-12}$& $1.20\textrm{e}{-12}$& $8.86\textrm{e}{-13}$ \\
        \bottomrule
    \end{tabular}
\end{table}

% Distance metric in the Lorentz model:
% \begin{equation*}
%     d^c_{\mathbb{L}}((t_1, x_1, y_1), (t_2, x_2, y_2)) = \sqrt{-2\left(\frac{1}{c} -t_1t_2 + x_1x_2 + y_1y_2\right)}
% \end{equation*}

\subsection{the Lorentz model operations}
The $n$-dimensional Lorentz model with curvature $-c$ is $\mathcal{L}^n_c$ where the manifold is $\{\rvx \in \R^{n+1} \mid \langle \rvx, \rvx \rangle_{\mathcal{L}_c} = -\frac{1}{c}\}$, where $\langle \rvx, \rvy \rangle_{\mathcal{L}_c}$ is the Lorentzian product computed as $\langle \rvx, \rvy \rangle_{\mathcal{L}_c} = -\rvx_0 \rvy_0 + \sum_{i=1}^n \rvx_i \rvy_i$.
% The Lorentzian norm is computed as $\Vert \rvv \Vert_{\mathbb{L}_c} = \s$
The exponential map of the Lorentz model is defined as:
\begin{equation}
% \label{eq:wrapped_normal}
    \exp_{\rvx}^c(\rvv) = \cosh(\alpha)\rvx + \sinh(\alpha) \frac{\rvv}{\alpha},
\end{equation}
and the log map of the Lorentz model is defined as:
\begin{equation}
    \log_{\rvx}^c(\rvy) = \frac{\cosh^{-1}(\beta)}{\sqrt{\beta^2 - 1}} (\rvy - \beta \rvx),
\end{equation}
where $\alpha = \sqrt{c\langle \rvv, \rvv \rangle_{\mathbb{L}_c}}$ and $\beta = -c\langle \rvx, \rvy \rangle_{\mathbb{L}_c}$.
